# Supplementary material for: Andreev Reflections in NbN/graphene Junctions under Large Magnetic Fields
Source: arXiv:2109.06285 source file (2021-09-13)
Supplement: Supplementary file 1 [file nl-2021-01072m_SI_Final_Version.pdf]

**Supplemental Materials**

**Andreev Reflections in NbN/graphene Junctions under Large Magnetic Fields**

Da Wang,[†,‡,⊥] Evan J. Telford,[†,⊥] Avishai Benyamini,[†,‡] John Jesudasan,[¶] Pratap Raychaudhuri,[¶] Kenji Watanabe,[§] Takashi Taniguchi,[§] James Hone,[‡] Cory R. Dean,[*,†] and Abhay N. Pasupathy[*,†,∥]

*†Department of Physics, Columbia University, New York, NY 10027, USA*
*‡Department of Mechanical Engineering, Columbia University, New York, NY 10027, USA*
*¶Tata Institute of Fundamental Research, Homi Bhabha Road, Colaba, Mumbai 400 005 India*
*§National Institute for Materials Science, 1-1 Namiki, Tsukuba, 305-0044 Japan*
*∥Condensed Matter Physics and Materials Science Department, Brookhaven National Laboratory, Upton, NY 11973, USA*
*⊥These authors contributed equally to this work*

***Fabrication Methods:***

The graphene Hall bar was shaped using an Oxford Plasmalab 100 ICP-RIE with a $CHF_3$:$O_2$ 40:4 sccm gas mixture with 60 W RF power and 40 mTorr gas pressure. Standard electron beam lithography techniques were used to define the contact geometry. Normal metal electrodes (Cr + Au 2 nm + 90 nm) were deposited using standard electron beam deposition techniques.

Thin films of NbN were synthesized through reactive dc magnetron sputtering by sputtering a Nb target in Ar-$N_2$ gas mixture. The substrate temperature is kept at 100 ºC, with an ambient pressure of 7 mTorr, and a target-to-substrate distance of 6.2 cm at a power of 220 W. The thickness of the NbN film is about 70-100 nm. The test sample films are grown on $SiO_2$ substrates and measured before deposition on actual devices. The test sample $T_{\mathrm{C}}$ is approximately 13 K.

***Transport Measurements:***

The data presented was measured utilizing a standard four-terminal lock-in technique. A low-frequency AC voltage generated by a lock-in amplifier is converted to an AC current using a large series resistor (1-10 MΩ) and the corresponding AC voltages (both NbN/g/Au and Au/g/Au channels) are measured at the same AC frequency along the sample. The current is sourced from the outer most Au electrode and drained into the NbN electrode. For equilibrium transport measurements (low excitation currents), when the system is in the Ohmic regime, $R = \frac{V_{\mathrm{AC}}}{I_{\mathrm{AC}}}$, where $I_{\mathrm{AC}}$ is the measured AC current and $V_{\mathrm{AC}}$ is the corresponding AC voltage. For non-equilibrium measurements, a DC+AC current bias scheme is used in which we superimpose a DC current bias $I_{\mathrm{DC}}$ onto the AC current excitation. The total current in such setup is: $I_{\mathrm{tot}} = I_{\mathrm{AC}} + I_{\mathrm{DC}}$. This is achieved by connecting the source lock-in amplifier in parallel with a DC voltage source. A 10 MΩ resistor is placed after the lock-in output and a 100 kΩ resistor is placed after the DC voltage source output. The AC current is measured with a lock-in at the AC source frequency and the DC current is measured with the DC voltage source. In this configuration $V_{\mathrm{AC}}$ is a measurement of the differential resistance $R_{\mathrm{AC}} = \frac{V_{\mathrm{AC}}}{I_{\mathrm{AC}}} = \frac{\mathrm{d}V}{\mathrm{d}I}$. An AC current excitation of ≈100 nA is used for all measurements.

***Fitting Zero-Field NbN/g/Au Junction Conductance to BTK Theory:***

To model the DC current dependence of the NbN/g/Au junction conductance in the RAR regime ($\epsilon_{\mathrm{F}} > \Delta_{\mathrm{NbN}}$), we use Blonder-Tinkham-Klapwijk theory[1]. The total current across the NbN/g interface is proportional to $1 + R(E) + AR(E)$ which is the incident electron probability minus the reflected electron probability $R(E)$ plus the Andreev reflection probability $AR(E)$. The total current can be calculated by integrating the total electron probability over all available electronic states, which is modeled by Fermi functions. We assume the graphene has a chemical potential of $\mu_{\mathrm{g}} = \mathrm{e}V$ and the NbN is grounded $\mu_{\mathrm{NbN}} = 0$.

$$\frac{I_{\mathrm{NS}}(V)}{I_{\mathrm{NN}}} = \frac{1+Z^2}{V} \int_{-\infty}^{\infty} [f(E-eV,T) - f(E,T)](1 + AR(E) - R(E))\mathrm{d}E \quad (S1)$$

Where $I_{\mathrm{NS}}$ is the current through the NbN/g/Au junction when the NbN is superconducting and $I_{\mathrm{NN}}$ is the current through the NbN/g/Au junction when the NbN is a normal metal. In our measurement in figure 1E, the sample temperature is much lower than the superconducting gap of NbN, so we can simplify equation (S1) taking the limit of $T \rightarrow 0$,

$$\frac{I_{\mathrm{NS}}(V)}{I_{\mathrm{NN}}} = \frac{1+Z^2}{V}(1 + AR(eV) - R(eV))\,V \quad (S2)$$

To compare the theory more directly to our experiment, we use equation (S2) to determine the differential conductance normalized to the normal state conductance.

$$\frac{G_{\mathrm{NS}}(V)}{G_{\mathrm{NN}}} = \frac{\mathrm{d}}{\mathrm{d}V} I_{\mathrm{NS}}(V) \cdot R_{\mathrm{NN}} = (1+Z^2)[1 + AR(eV) - R(eV)] \quad (S3)$$

The original BTK derivation omits the role of energy broadening in the density of states. We can easily include the role of broadening by introducing a finite quasiparticle scattering lifetime $\frac{1}{\Gamma}$ and substituting $E \rightarrow E + i\Gamma$ in the expression for $R(E)$ and $AR(E)$[1].

***Modeling NbN/g/Au Junction Conductance in the QH Regime:***

In the quantum Hall regime, we use the Büttiker formalism to calculate the SC/g junction conductance. We expect the contribution to the conductance from Andreev processes to be a summation of available Andreev bound states crossing the Fermi level:

$$G_{\mathrm{AR}} = \frac{\mathrm{e}^2}{\pi\hbar}\sum_{1}^{\mathrm{n}^*} B_{\mathrm{n}} \quad (S4)$$

$B_{\mathrm{n}}$ is the hole probability. For this work, we focus specifically on the $\nu = 4$ quantum Hall state in which the conductance can be simplified to:

$$G_{\mathrm{AR}} = \frac{\mathrm{e}^2}{\pi\hbar}\sum_{1}^{4} B_{\mathrm{n}} = \frac{2\mathrm{e}^2}{\pi\hbar}\frac{q^2/(1-\gamma_0^2)}{1+\sqrt{1-q^2/(1-\gamma_0^2)}} \quad (S5)$$

$q = \frac{2s}{(s^2+w^2+1)}$ and $\gamma_0 = \frac{[s^2+w^2-1]*\sin\left(\frac{\pi\nu}{2}\right)+2w\cos\left(\frac{\pi\nu}{2}\right)}{s^2+w^2+1}$. The interfacial scattering parameter is defined as $w = \left[\frac{2m_{\mathrm{N}}U_0^2}{\hbar^2\varepsilon_{\mathrm{F}}^{(\mathrm{N})}}\right]^{\frac{1}{2}}$(where $m_N$ is the electron mass, $U_0$ is the interfacial scattering potential, and $\epsilon_{\mathrm{F}}$ is the Fermi level of graphene) and the Fermi velocity mismatch parameter is $s = [\varepsilon_{\mathrm{F}}^{(\mathrm{S})}m_{\mathrm{N}}]/[\varepsilon_{\mathrm{F}}^{(\mathrm{N})}m_{\mathrm{S}}]$. In the main text, we extract the scattering parameter $w$ from our data through the following procedure:

(1) Extract minimum conductance within the $\nu = 4$ plateau and determine the hole probability $B_{\mathrm{n}}$ using equation (S4).

(2) Using equation (S5), we can determine $w$ from the hole probability $B_{\mathrm{n}}$ (figure S11A).

To understand the field dependence of *w*, we need only examine the field dependence of the cyclotron frequency $\omega_{\mathrm{c}} = \frac{\mathrm{e}B}{m\mathrm{c}}$. As perpendicular field increases, the cyclotron frequency increases. For a given filling factor $\nu = 2\varepsilon_{\mathrm{F}}^{(\mathrm{N})}/(\hbar\omega_{\mathrm{c}})$, $\varepsilon_{\mathrm{F}}^{(\mathrm{N})}$ is larger at higher fields due to the larger cyclotron motion frequency, resulting in smaller *w* at higher magnetic fields (figure S11B).

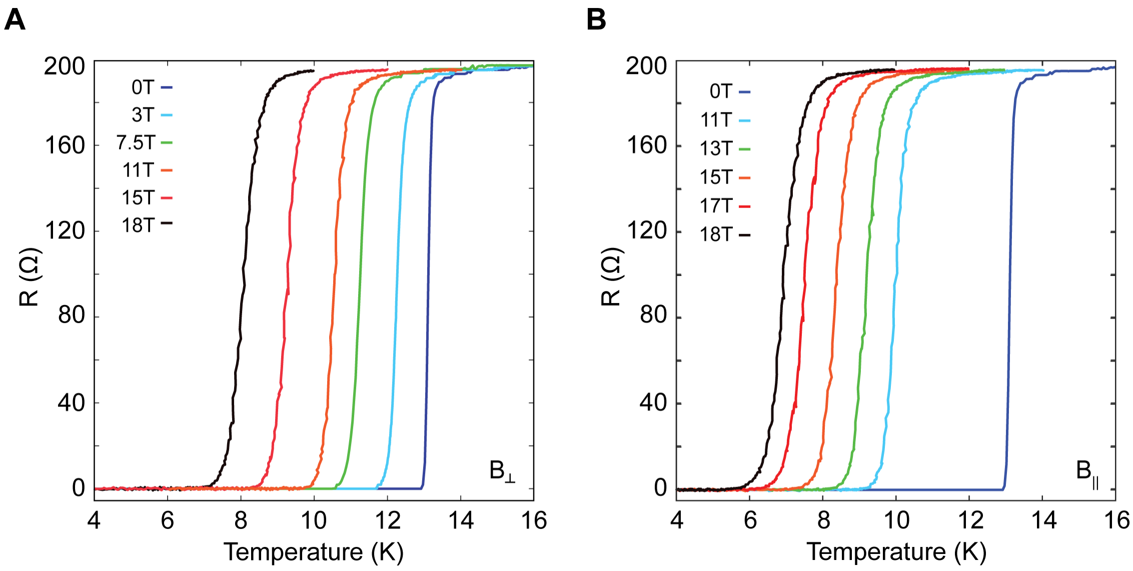


Figure S1. Superconducting properties of NbN. A,B) 4-terminal longitudinal NbN resistance versus temperature for various magnetic fields perpendicular (A) and parallel (B) to the sample plane. Results are consistent with expectations from supplemental reference[2].

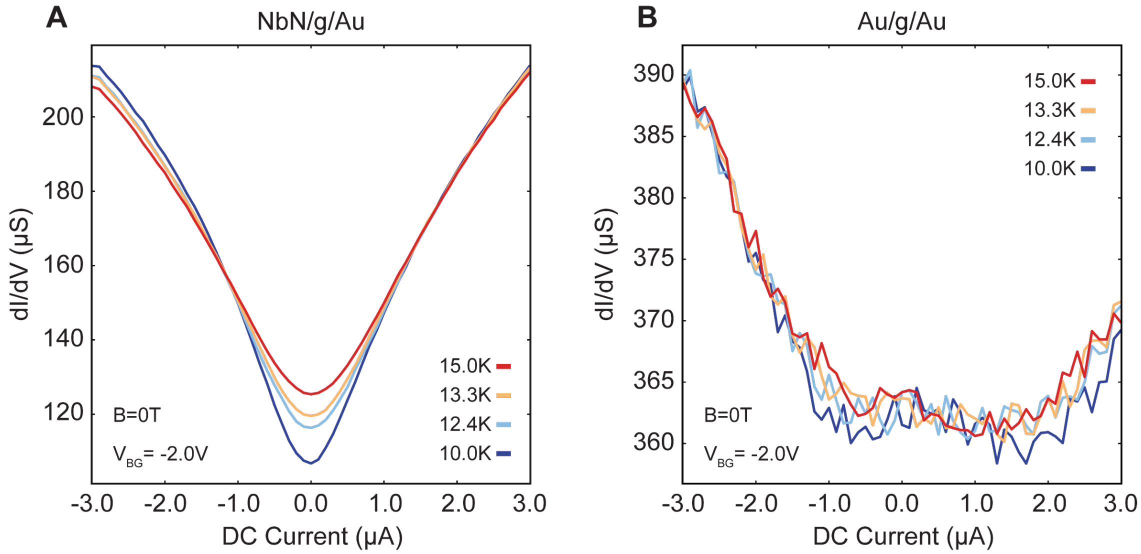


Figure S2. Temperature dependence of NbN/g/Au and Au/g/Au channel conductances. Differential NbN/g/Au (A) and Au/g/Au channel (B) conductance versus DC current bias for various temperatures across the NbN superconducting transition temperature ($T_C \approx$ 13.2 K). The Au/g/Au channel is temperature independent across $T_C$, whereas the NbN/g/Au channel develops a zero-bias conductance dip and an increase in conductance for large biases for $T < T_C$ due to the emergence of Andreev reflection processes[3,4].

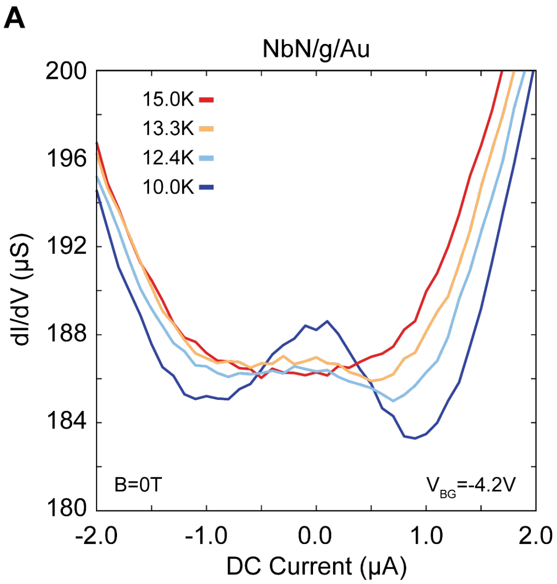


Figure S3. Temperature dependence of NbN/g/Au and Au/g/Au channel conductances. Differential NbN/g/Au (A) and Au/g/Au channel (B) conductance versus DC current bias for various temperatures across the NbN superconducting transition temperature ($T_C \approx$ 13.2 K). The Au/g/Au channel is temperature independent across $T_C$, whereas the NbN/g/Au channel develops a zero-bias conductance peak for $T < T_C$ due to the emergence of Andreev reflection processes[3,4].

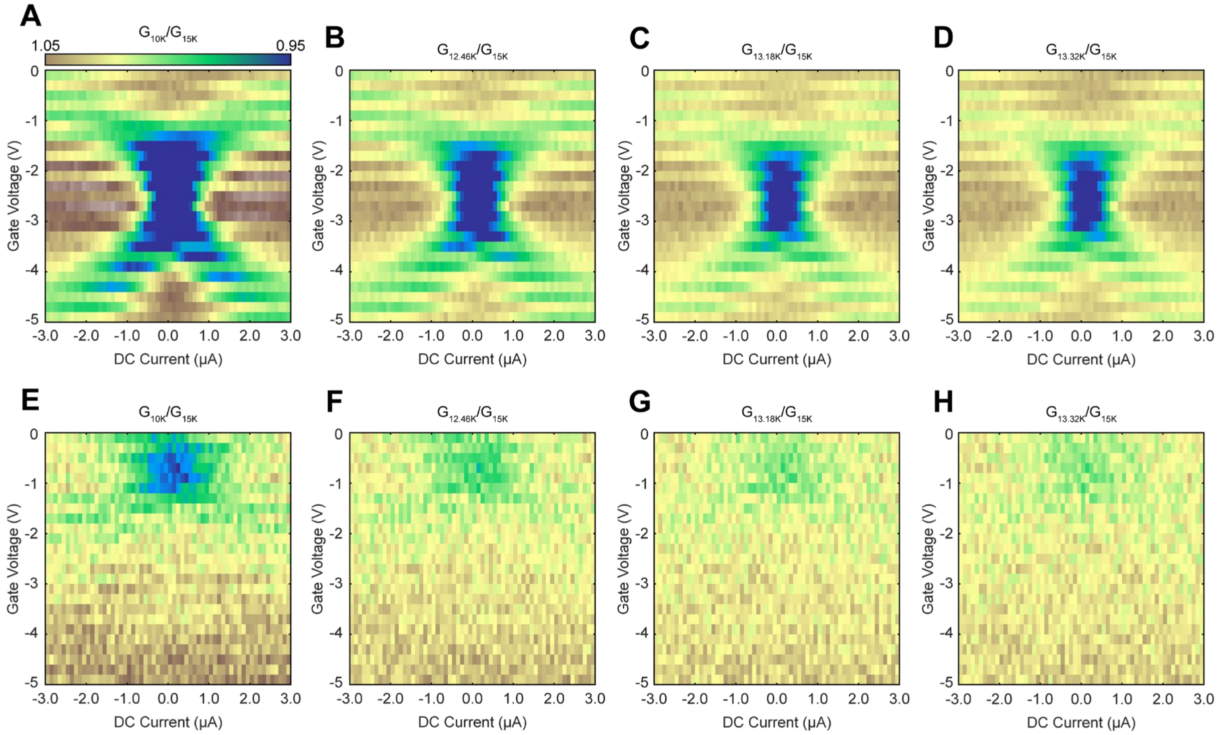


Figure S4. NbN/g/Au and Au/g/Au channel conductance maps across $T_C$. A-D) 2D color maps of differential NbN/g/Au channel conductance versus DC bias and back-gate voltage at 10 K (A), 12.46 K (B), 13.16 K (C), and 13.32 K (D). Each 2D color map is normalized by the 2D map taken at 15 K. The conductance enhancement at finite bias near the CNP (specular Andreev reflections) and the “cross” shaped feature become more prominent as temperature is lowered below the $T_C$ of NbN[3,4]. E-H) 2D color maps of differential Au/g/Au channel conductance versus DC bias and back-gate voltage at 10 K (E), 12.46 K (F), 13.16 K (G), and 13.32 K (H). Each 2D color map is normalized by the 2D map taken at 15 K.

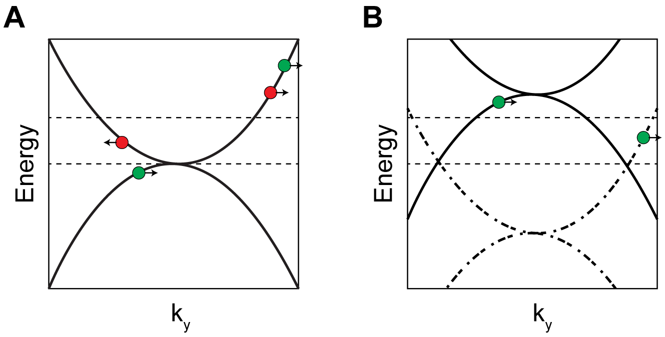


Figure S5. Specular Andreev reflection at zero bias. A) Cartoon of Andreev reflection processes at zero magnetic field. The graphene band structure is shown by the solid black lines. The two points in red correspond to intraband (retro) Andreev reflection processes, while the two points in green correspond to interband (specular) Andreev reflection processes. B) Cartoon of Andreev reflection processes at a finite parallel magnetic field. The dispersion for up-spin (solid black lines) and down-spin (dotted black lines) have the CNP's well separated energetically. Interband Andreev processes can occur at zero applied bias[5]. In both plots, dashed black lines denote the chemical potential and zero-field CNP.

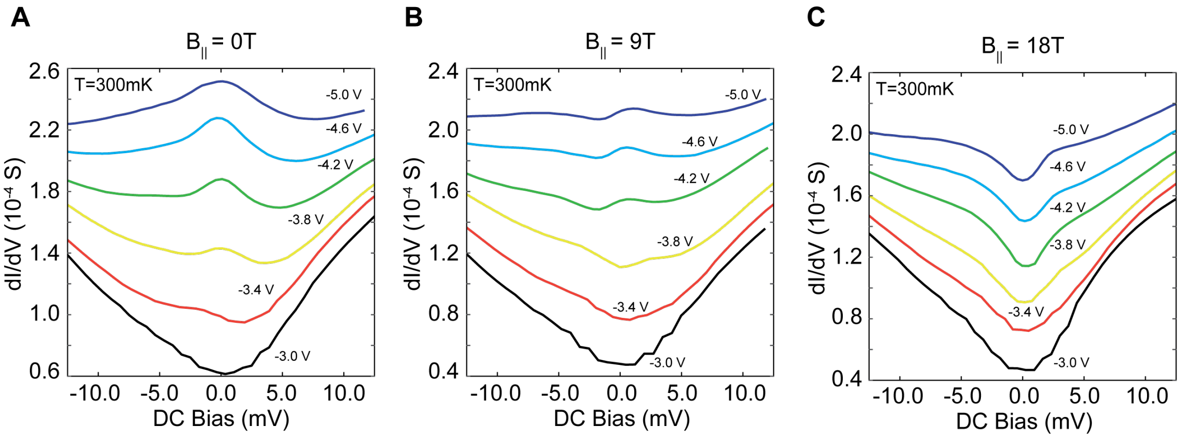


Figure S6. Elimination of conductance features with parallel magnetic field. Differential NbN/g/Au conductance versus DC voltage bias at various back-gate voltages for 0 T (A), 9 T (B), and 18 T (C) parallel magnetic fields. At zero magnetic field, as the back-gate voltage is swept away from the CNP, we observe three distinct tunneling regimes. At $V_{\mathrm{BG}}$ = -3.0 V, the Fermi level of graphene is at the CNP, manifesting a conductance dip near zero bias. At $V_{\mathrm{BG}}$ = -4.2 V, a zero-bias conductance peak emerges due to Andreev processes saddled by conductance minima corresponding to the condition where $\mathrm{e}|V_{\mathrm{NS}}| = \epsilon_{\mathrm{F}}$ . At $V_{\mathrm{BG}}$ = -5.0 V, the conductance minima disappear as the CNP is outside of the NbN superconducting gap and the graphene acts as a normal metal. As parallel magnetic field is increased, the conductance dips and zero-bias peaks disappear for any back-gate voltage due to Zeeman splitting of the graphene band structure[5] and a reduction of the superconducting gap of NbN. To determine Zeeman splitting in the bilayer graphene, we extract the relative positions of conductance dips for a given $V_{\mathrm{BG}}$ at different fields: e.g. at $V_{\mathrm{BG}}$= -4.2 V, the conductance dips move from ≈ 4.7 meV at 0 T, to ≈ 4.2 meV at 4.5 T to ≈ 3.6 meV at 9 T. This corresponds to a ≈ 1.1 meV Zeeman shift induced by 9 T parallel field, which gives a $g$ factor ≈ 2.1.

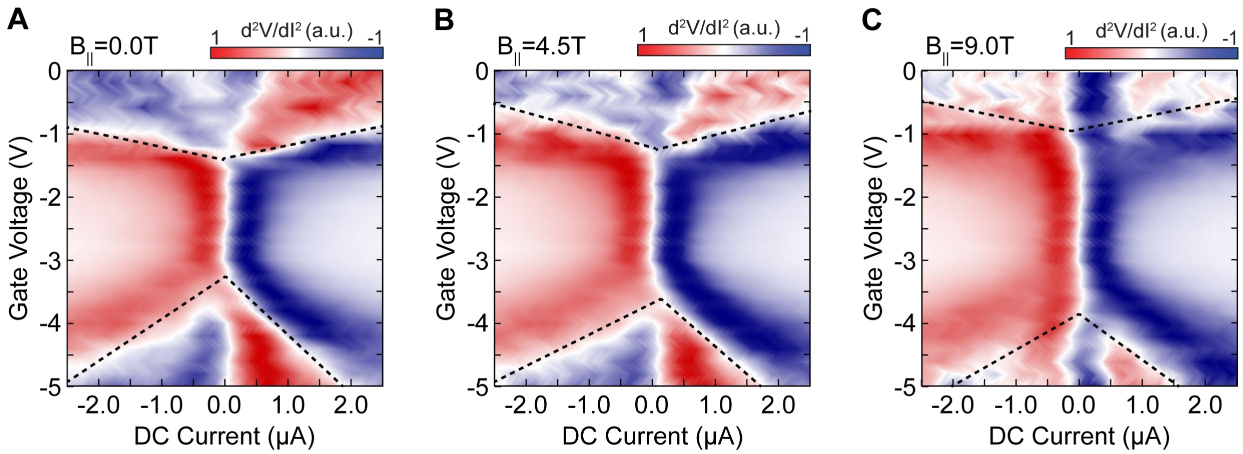


Figure S7. Movement of the RAR/SAR boundary with parallel magnetic field. Derivative of junction resistance versus back-gate voltage and DC current bias for 0 T (A), 4.5 T (B), and 9.0 T (C) parallel magnetic fields. The boundary between RAR and SAR processes are denoted by black dashed lines[3,4]. At zero magnetic field, the position of the RAR/SAR crossover at zero DC bias is proportional to the disorder broadening in the NbN/g junction as the crossovers should intersect at the CNP. At finite fields, the position of the RAR/SAR crossover broadens due to the spin splitting of the graphene band structure[5].

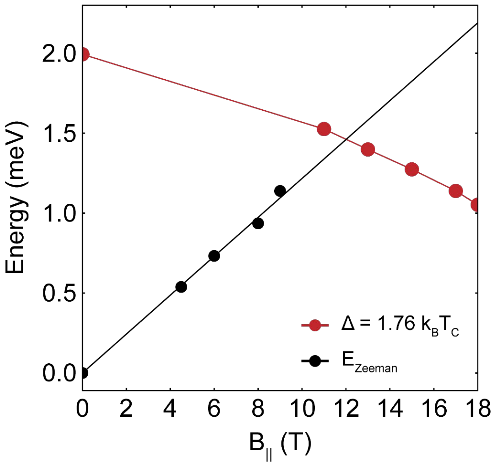


Figure S8. Evolution of Zeeman energy and NbN superconducting gap versus parallel magnetic field. Calculation of the superconducting gap of NbN (red dots and solid red line) and the extracted Zeeman splitting in bilayer graphene (black dots) and the corresponding fit (solid black line) versus parallel magnetic field. The bilayer graphene Zeeman splitting becomes larger than the superconducting gap of NbN at ~12 T.

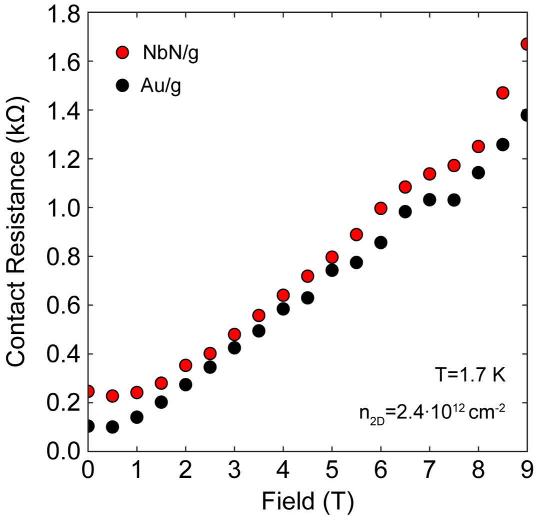


Figure S9. Contact resistances versus perpendicular magnetic field. NbN/g (red dots) and Au/g (black dots) contact resistances versus perpendicular magnetic field. The contact resistances are determined by measuring the 2-terminal NbN/g/Au and Au/g/Au resistances at a graphene density of $n_{2D}$ = 2.4·$10^{12}$ cm$^{-2}$ and subtracting the fridge line resistances. Contact resistances were extracted at 1.7 K.

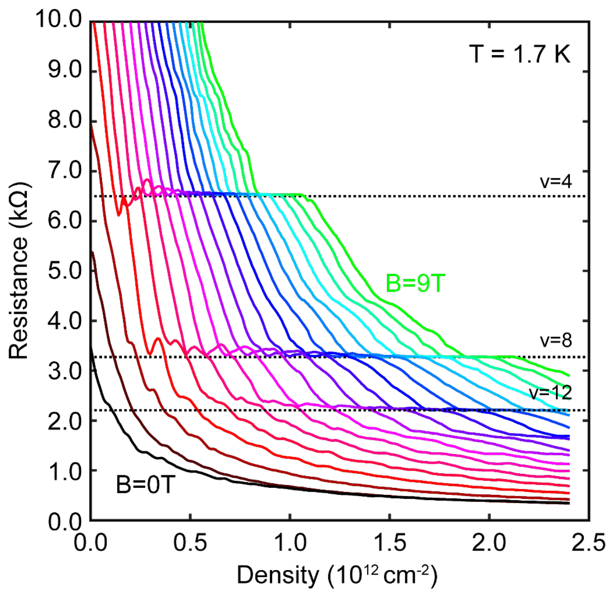


Figure S10. Fan diagram of the graphene channel. Au/g/Au channel resistance versus electronic carrier density at various magnetic fields. Observed well-quantized quantum Hall plateaus are denoted by dashed black lines.

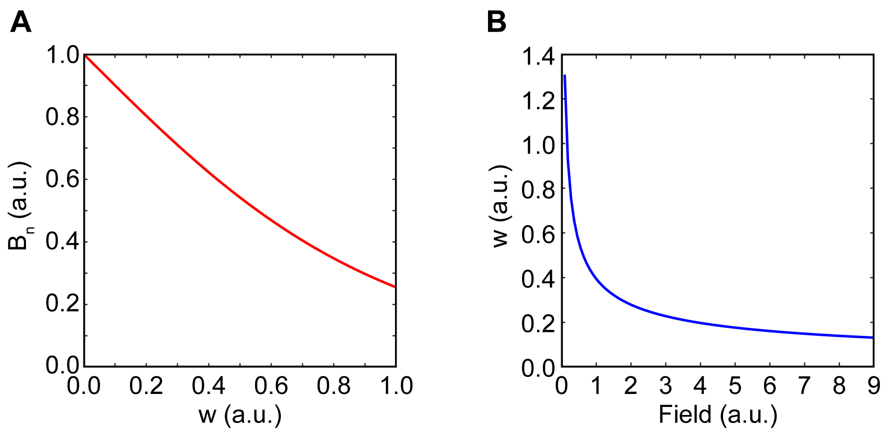


Figure S11. Calculation of SC/g interface parameters. A) Calculated hole probability $B_{\mathrm{n}}$ versus scattering parameter $w$ assuming $s$ = 1. B) Scattering parameter $w$ versus magnetic field. All calculations were done using equations derived in reference[6].

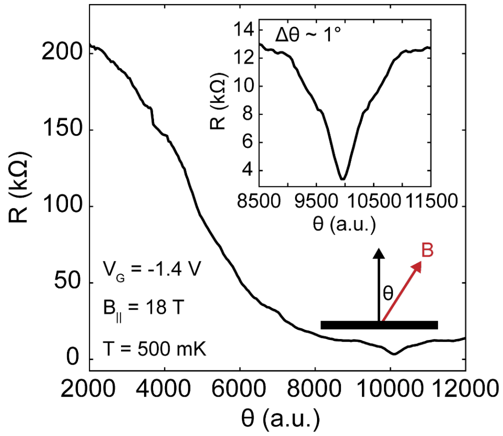


Figure S12. Calibrating the magnetic field direction. Resistance of the Au/g/Au channel versus sample rotator angle at 18 T and 500 mK with an applied back-gate voltage of -1.4 V (near the CNP). Inset shows a zoom in of the Au/g/Au channel resistance versus angle near 90º. The graphene resistance is minimized (maximized) when the magnetic field is oriented along the in-plane (out-of-plane) direction.

**Supplemental References:**

(1) Blonder, G. E.; Tinkham, M.; Klapwijk, T. M. Transition from Metallic to Tunneling Regimes in Superconducting Microconstrictions: Excess Current, Charge Imbalance, and Supercurrent Conversion. *Phys. Rev. B* **1982**, *25* (7), 4515–4532. https://doi.org/10.1103/PhysRevB.25.4515.

(2) Mondal, M.; Chand, M.; Kamlapure, A.; Jesudasan, J.; Bagwe, V. C.; Kumar, S.; Saraswat, G.; Tripathi, V.; Raychaudhuri, P. Phase Diagram and Upper Critical Field of Homogeneously Disordered Epitaxial 3-Dimensional NbN Films. *J. Supercond. Nov. Magn.* **2011**, *24* (1–2), 341–344. https://doi.org/10.1007/s10948-010-1038-8.

(3) Efetov, D. K.; Efetov, K. B. Crossover from Retro to Specular Andreev Reflections in Bilayer Graphene. *Phys. Rev. B* **2016**, *94* (7), 075403. https://doi.org/10.1103/PhysRevB.94.075403.

(4) Efetov, D. K.; Wang, L.; Handschin, C.; Efetov, K. B.; Shuang, J.; Cava, R.; Taniguchi, T.; Watanabe, K.; Hone, J.; Dean, C. R.; Kim, P. Specular Interband Andreev Reflections at van Der Waals Interfaces between Graphene and NbSe2. *Nat. Phys.* **2016**, *12* (4), 328–332. https://doi.org/10.1038/nphys3583.

(5) Soori, A.; Sahu, M. R.; Das, A.; Mukerjee, S. Enhanced Specular Andreev Reflection in Bilayer Graphene. *Phys. Rev. B* **2018**, *98* (7), 075301. https://doi.org/10.1103/PhysRevB.98.075301.

(6) Hoppe, H.; Zülicke, U.; Schön, G. Andreev Reflection in Strong Magnetic Fields. *Phys. Rev. Lett.* **2000**, *84* (8), 1804–1807. https://doi.org/10.1103/PhysRevLett.84.1804.
